# Supplementary material for: Room-temperature superconductivity in an artificial 2D Mott-insulating square lattice and its advanced condensed phase that generates a low-loss current in the atmosphere: A possible perpetual motion machine
Source: arXiv:2012.15858 ancillary file (2020-12-31)
Supplement: Supplementary file 1 [file SupplementaryMaterial_Zen.pdf]

# Supplementary Material

**Room-temperature superconductivity in an artificial 2D Mott-insulating square lattice and its advanced condensed phase that generates a low-loss current in the atmosphere : A possible perpetual motion machine on the back of spontaneous symmetry breaking**

Nobuyuki Zen*

**This PDF file includes:**

Materials and Methods

Figs. S1 – S11

Tables S1 – S4

MFM Results

Full Reference List

* Corresponding author. E-mail: n.zen@aist.go.jp

ORCiD: https://orcid.org/0000-0003-4897-478X

**Materials and Methods**

***PnC–Nb fabrication*****:** An $SiO_2$ sacrificial layer of 1.0-μm thickness was deposited on a p-type Si wafer, of thickness, diameter, and orientation of 0.4 mm, 76.0 mm, and (100), respectively, by chemical vapor deposition (PD-270STL, Samco) with the stage temperature kept at 80°C. The pressure of the mixture of gases of TEOS (tetraethoxysilane) and $O_2$ was 30 Pa, and the total deposition time was 42 minutes. Post deposition, a Nb film of 150-nm thickness was deposited on the $SiO_2$ layer by sputtering (M12-0130, Science Plus) at 10°C, using Ar gas at 1.0 Pa, for 130 s. Subsequently, an i-line chemical resist (PFi-245, Sumitomo Chemical) was spin-coated to be a thickness of 300 nm on the Nb layer, and PnC patterns were formed using an i-line stepper (NSR-2205i12D, Nikon TEC) with an exposure time of 350 ms. The exposed region of the Nb layer was removed by reactive ion etching (RIE-10NR, Samco) using $SF_6$ gas at 10.0 Pa for a total etching time of 210 s. Sample chips were prepared, by cutting the resulting wafer into $5 \times 5$ mm$^2$ squares using a dicing machine (DAD522, DISCO), and a protective chemical resist (PFi-68A7, Sumitomo Chemical) was removed. Finally, the $SiO_2$ sacrificial layer underneath the Nb layer was removed by an HF dry etcher (memsstar®SVR™ vHF, Canon). The sample chips were exposed under a mixture of 250-sccm HF gas and water vapor, which consisted of 100-sccm $N_2$ and 10-mg $H_2O$, with the stage temperature kept at 5°C for durations of 120 s and 360 s for an 8-Torr step and subsequent 9-Torr step, respectively. The suspended Nb structure was inspected using a laser microscope (LEXT OLS4000, Olympus).

The GDSII file of the i-line mask pattern used for fabricating the PnC–Nb in this study is available in the open-access repository Dryad.[28]

***R–T measurements*****:** All *R*–*T* measurements in Figs. 1(d), 2, and 6 were performed using the PPMS (Quantum Design) in zero magnetic field ($\mu_0 H_\perp \leq 10$ μT), and the sample space was kept at a low pressure of approximately 200 Pa. The PnC–Nb chips were mounted on a PPMS sample puck using vacuum grease (Apiezon N, M&I Materials). Electrical contacts of the sample to the PPMS puck were made by aluminum wire bonding, and the resistance was measured by the four-probe method using electrical pads as denoted in Fig. 1(b). The PPMS was operated in the AC drive mode using the standard calibration mode, and the number of readings taken was 25; that is, at each temperature, a positively and negatively oscillating 8.33-Hz square-wave excitation current of amplitude of ±10 μA was repeatedly applied to the sample 25 times, and the measured voltage

was obtained by averaging the absolute values to eliminate errors from DC offset voltages. The complete cooling–warming procedures of the *R*–*T* cycles in this study are shown in Tables S1–S4.

***Electrical measurements in the PPMS*****:** The electrical properties of the RTSCs and SCRQ shown in Figs. 3, 4, and 7(a) were measured in the PPMS at 300 K and at a low pressure of approximately 200 Pa. All measurements, except the critical magnetic field measurement in Fig. 3, were performed in zero magnetic field ($\mu_0 H_\perp \leq 10$ μT). All measurements were executed by sweeping the current using the four-probe method as denoted in Fig. 1(b). To obtain Fig. 3, the delta mode (6221/2182A combination, Keithley) was externally connected to the PPMS to minimize constant thermoelectric offsets; specifically, a current pulse with a width of 10 ms and a period of 100 ms was applied, and the voltage was measured in the minimum range of 10 mV. To obtain Fig. 4, an SMU (B2911A, Keysight) was externally connected to the PPMS, and the voltage was measured while the direct current was swept. To obtain Fig. 7(a), the resistance bridge board installed in the PPMS was used, which was operated in the DC drive mode, and the number of readings taken was 10; specifically, the applied 8.33-Hz square-wave current was not reversed at each current point, and the voltage was obtained by averaging two consecutive values.

***Electrical measurements in the atmosphere*****:** All experimental data shown in Figs. 8 and 9 were obtained in the atmosphere (i.e., at room temperature, in a terrestrial magnetic field, and under atmospheric pressure). To obtain the *C*–*V* results in Fig. 8(a), a semiconductor-characterization system (B1500A, Keysight) was connected to the SCRQ as indicated in the inset. To obtain Fig. 8(b), the SMU was connected to the SCRQ using the four-probe method as indicated in the inset. To obtain Fig. 9(b), a nanovoltmeter (2182A, Keithley) was connected as indicated in the inset of Fig. 9(a). The load resistors were commercial metal film resistors. Prior to the measurements, a discharge test of an alkaline button cell (LR44, Panasonic) was performed to verify the experimental setup. The serially connected $R_L$ was 100 Ω, and the value of $V_L$, which was initially 1.5 V, decreased considerably after approximately 5 hours; thus, the discharge completed as expected, and the experimental setup was verified [details can be referred from Fig. S4].

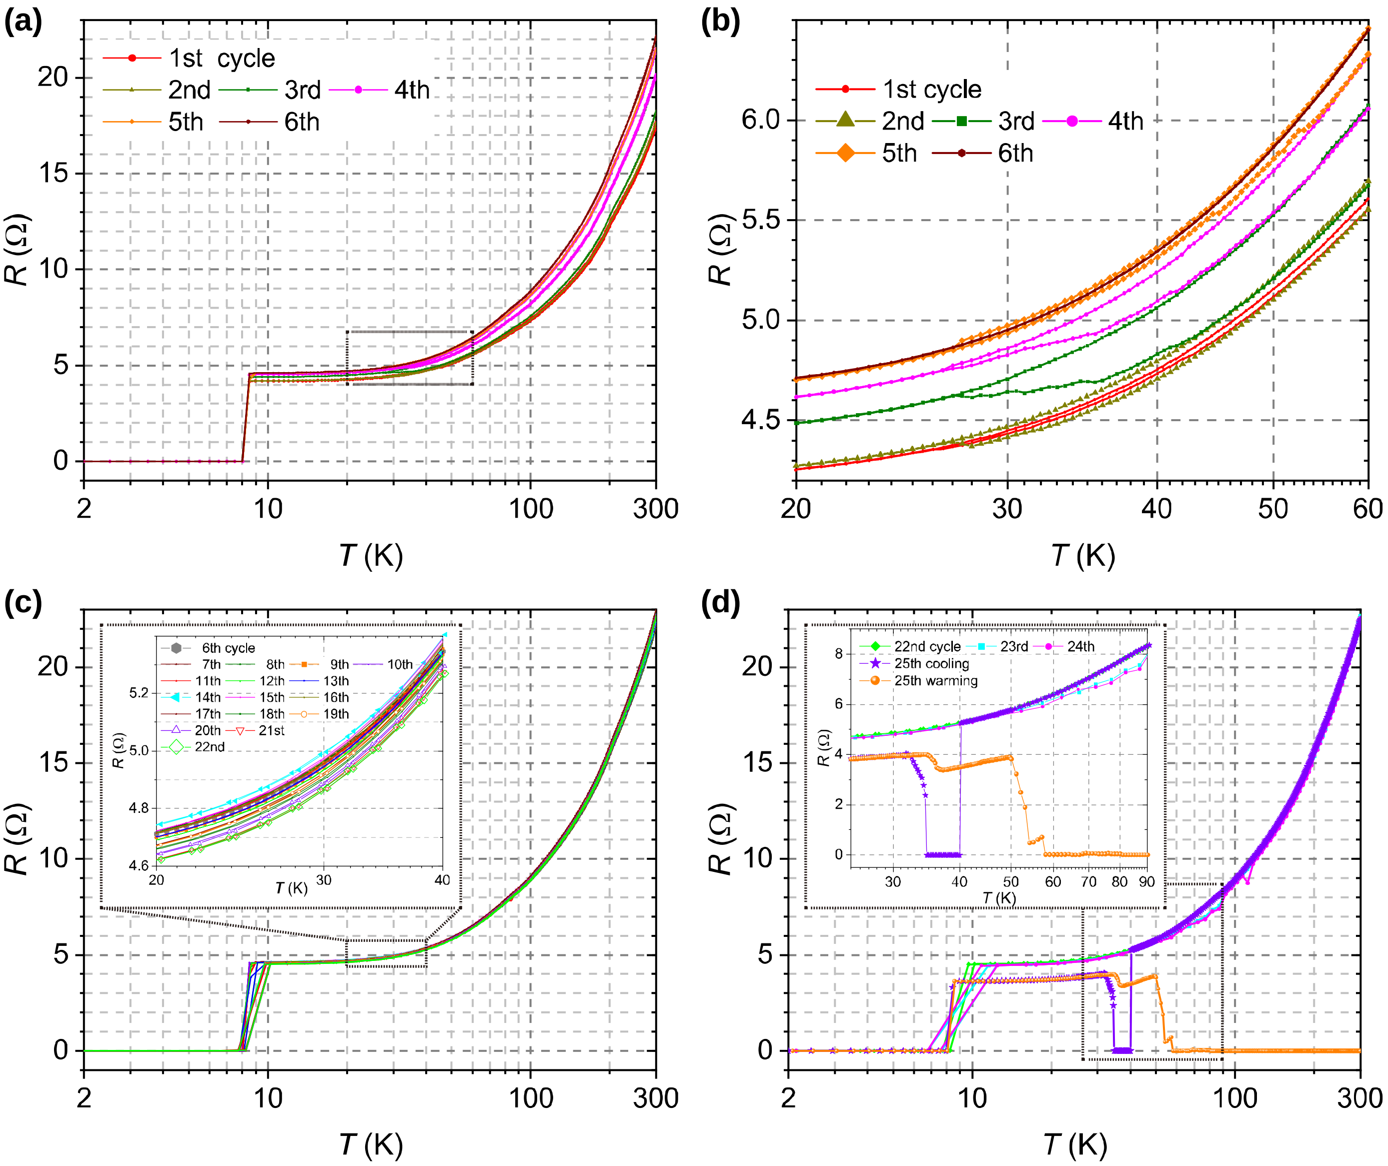


**Figure S1. All *R*–*T* cycles to make the RTSC shown in Fig. 2.** (**a**) First to sixth temperature cycles. (**b**) Zoomed-in plot of the region surrounded by the black dashed square in (a). An abnormal increase in the resistance is confirmed between 20 K and 60 K for the first five cycles; for each cycle, the warming curve does not retrace the cooling curve. (**c**) Sixth to 22nd cycle. As shown in the inset, the obvious non-retraced behavior is lost for each temperature cycle, but the entire *R*–*T* curve goes up and down. (**d**) The rest of the temperature cycles to realize the RTSC. Inset, zoomed-in plot. In the 23rd and 24th cycles, just before the RTSC is realized, *R*–*T* curves exhibit unstable behavior at high temperatures (50–120 K), which is the sign of the RTSC. The raw data of all *R*–*T* curves is available in the open-access repository Dryad.[28] See Table S1 for the cooling–warming procedures of this measurement.

**Table S1. Cooling–warming procedures to make the RTSC shown in Fig. 2**

| Cycle number | Cooling–warming rate and temperature approaching mode* | | Elapsed time |
|---|---|---|---|
| 1st ~ 11th | 300 → 60 K: 1 K/min | S | 18 ~ 20 hrs/cycle |
| | 60 → 2 K: 0.5 K/min | F | |
| | 2 → 60 K: 0.5 K/min | F | |
| | 60 → 300 K: 1 K/min | S | |
| 12th ~ 13th | 300 → 2 K: 1 K/min | S | 9 ~ 10 hrs/cycle |
| | 2 → 300 K: 1 K/min | S | |
| 14th ~ 21st | 300 → 2 K: 2 K/min | S | 5 ~ 6 hrs/cycle |
| | 2 → 300 K: 2 K/min | S | |
| 22nd | 300 → 2 K: 2 K/min | S | 4.8 hrs |
| | 2 → 230 K: 2 K/min | S | |
| | 230 → 300 K: 5 K/min | S | |
| 23rd ~ 24th | 300 → 2 K: 5 K/min | S | 2 ~ 3 hrs/cycle |
| | 2 → 300 K: 5 K/min | S | |
| 25th | 300 → 50 K: 1 K/min | S | 18.0 hrs |
| | 50 → 25 K: 0.25 K/min | F | |
| | 25 → 2 K: 0.5 K/min | S | |
| | 2 → 25 K: 0.5 K/min | S | |
| | 25 → 50 K: 0.25 K/min | F | |
| | 50 → 300 K: 1 K/min | S | |

We performed the measurements in zero magnetic field using the physical property measurement system (PPMS, Quantum Design). The PPMS was operated in the AC drive mode using the standard calibration mode. The amplitude of the square-wave excitation current was ±10 μA. At each resistance measurement, the number of readings was 25. See Materials and Methods section "*R–T measurements*" for details.

*Letters "S" and "F" after each cooling–warming rate indicate that the resistance is measured by sweeping or fixing the temperature, respectively.

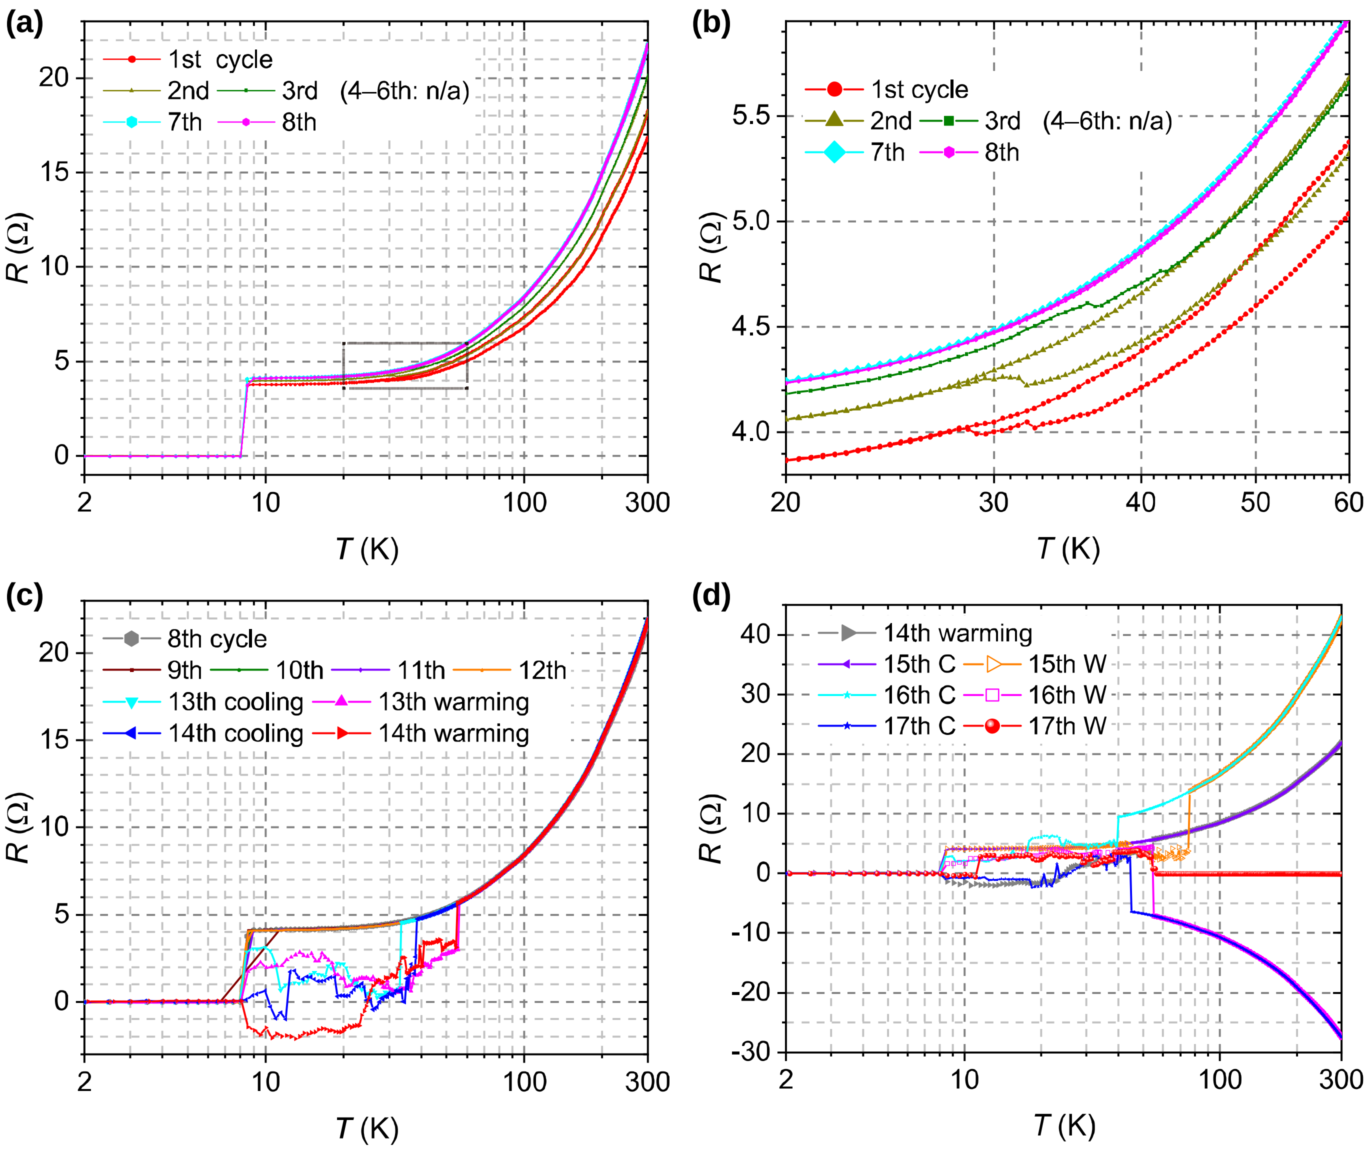


**Figure S2. All *R*–*T* cycles to make the RTSC used in Fig. 3.** By applying a perpendicular magnetic field of $\mu_0 H_\perp$ = 1–2 mT, 17 temperature cycles were performed. (**a**) First to eighth temperature cycles. In the middle of the third cooling process to the end of the sixth warming process, the resistance was lost owing to the disconnection of bonded wires. Prior to the seventh cycle, they were repaired. (**b**) Zoomed-in plot of the region surrounded by the black dashed square in (a). An abnormal increase in the resistance is confirmed between 20 K and 60 K, which is the same as for the sample in Fig. S1(b). (**c**) Eighth to 14th cycles. (**d**) The rest of the temperature cycles to realize the RTSC. The complicated *R*–*T* curves might be due to the applied magnetic field during the measurements. The most curious behavior is the negative *R*–*T* curves observed after the 16th warming process. Although further investigations will be performed in the future, we deduce that the insufficient balance of charges in the specimen is exposed by the external magnetic field. The subsequent 17th cooling process traces the same negative *R*–*T* curve. Finally, during the 17th warming process (red), the resistance decreases to zero between 50 K and 60 K, and the zero-resistance state remains up to 300 K. See Table S2 for the cooling–warming procedures of this measurement.

**Table S2. Cooling–warming procedures to make the RTSC used in Fig. 3**

| Cycle number | Cooling–warming rate and temperature approaching mode[*] | | External magnetic field (mT) | Amplitude of excitation current (μA) | Elapsed time |
|---|---|---|---|---|---|
| 1st ~ 2nd | 300 → 60 K: 1 K/min | S | 1 | 10 | 18 ~ 19 hrs/cycle |
| | 60 → 2 K: 0.5 K/min | F | | | |
| | 2 → 60 K: 0.5 K/min | F | | | |
| | 60 → 300 K: 1 K/min | S | | | |
| 3rd | 300 → 60 K: 1 K/min | S | 1 | 10 | 18.9 hrs |
| | 60 → 2 K: 0.5 K/min | F | | | |
| | 2 → 60 K: 0.5 K/min | F | | n/a[†] | |
| | 60 → 300 K: 1 K/min | S | | | |
| 4th ~ 6th | 300 → 60 K: 1 K/min | S | 1 | n/a[†] | 18 ~ 20 hrs/cycle |
| | 60 → 2 K: 0.5 K/min | F | | | |
| | 2 → 60 K: 0.5 K/min | F | | | |
| | 60 → 300 K: 1 K/min | S | | | |
| Six days intervals: during the period, bonded wires were repaired. | | | | | |
| 7th ~ 8th | 300 → 60 K: 1 K/min | S | 2 | 10 | 18 ~ 20 hrs/cycle |
| | 60 → 2 K: 0.5 K/min | F | | | |
| | 2 → 60 K: 0.5 K/min | F | | | |
| | 60 → 300 K: 1 K/min | S | | | |
| 9th | 300 → 195 K: 1 K/min | S | 2 | 10 | 13.3 hrs |
| | 195 → 2 K: 5 K/min | S | | | |
| | 2 → 25 K: 0.5 K/min | S | | | |
| | 25 → 60 K: 0.25 K/min | F | | | |
| | 60 → 300 K: 1 K/min | S | | | |
| Two weeks intervals: during the period, the sample was kept in a laboratory environment. | | | | | |
| 10th ~ 17th | 300 → 60 K: 1 K/min | S | 2 | 100 | 16 ~ 18 hrs/cycle |
| | 60 → 20 K: 0.5 K/min | F | | | |
| | 20 → 2 K: 0.5 K/min | S | | | |
| | 2 → 20 K: 0.5 K/min | S | | | |
| | 20 → 60 K: 0.5 K/min | F | | | |
| | 60 → 300 K: 1 K/min | S | | | |

We performed the measurements using the PPMS. The PPMS was operated in the AC drive mode using the standard calibration mode. The amplitude of the square-wave excitation current was ±10 μA until the 9th temperature cycle. After the 10th cycle, the amplitude was changed to ±100 μA. For each resistance measurement, the number of readings was 25. See Materials and Methods section "*R–T measurements*" for details.

[*]Letters "S" and "F" after each cooling–warming rate indicate that the resistance is measured by sweeping or fixing the temperature, respectively.

[†]The excitation current was not applied to the sample owing to the disconnection of bonded wires.

**Table S3. Cooling–warming procedures for Fig. 6 which results in the SCRQ**

| Cycle number | Cooling–warming rate and temperature approaching mode* | | Elapsed time |
|---|---|---|---|
| 1st ~ 2nd | 300 → 60 K: 2 K/min | S | 14 ~ 15 hrs/cycle |
| | 60 → 20 K: 0.5 K/min | F | |
| | 20 → 2 K: 0.5 K/min | S | |
| | 2 → 20 K: 0.5 K/min | S | |
| | 20 → 60 K: 0.5 K/min | F | |
| | 60 → 300 K: 1 K/min | S | |

We performed the measurements in zero magnetic field using the PPMS. The PPMS was operated in the AC drive mode using the standard calibration mode. The amplitude of the square-wave excitation current was ±10 μA. At each resistance measurement, the number of readings was 25. See Materials and Methods section "*R–T measurements*" for details.

*Letters "S" and "F" after each cooling–warming rate indicate that the resistance is measured by sweeping or fixing the temperature, respectively.

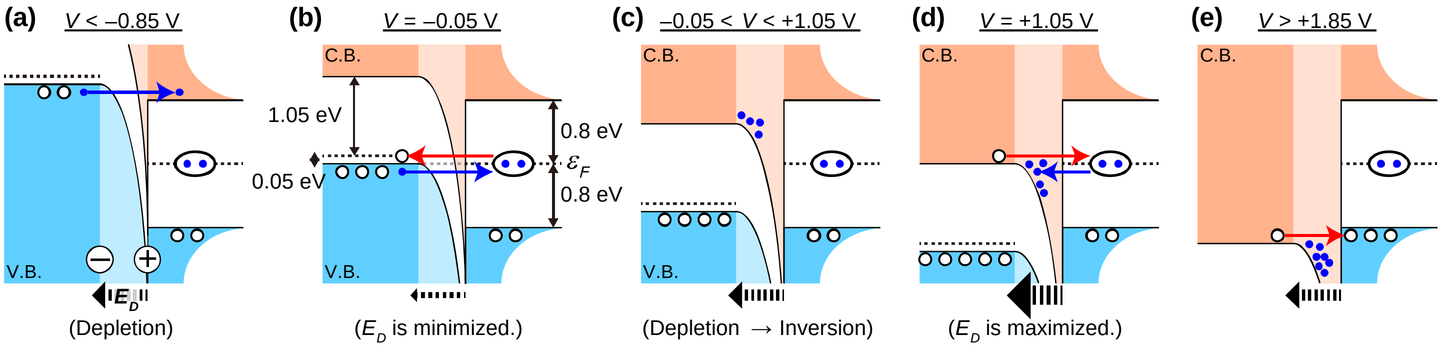


**Figure S3. Semiconductor model of the SCRQ in various bias regions.** The built-in electric field $E_D$ created at the p-Semi–SC interface is denoted by the broken arrow: direction, polarity; width, strength. (**a**) The edge level of the valence band (V.B., shaded in light blue) of the p-Semi is higher than that of the conduction band (C.B., shaded in light orange) of the SC. Therefore, an electron (blue dot) at the V.B. of the p-Semi is transported to an empty state at the C.B. of the SC (blue arrow). The tunneling process is ohmic,[21] which is consistent with the *dI/dV* result at $V <$ –0.85 V [Fig. 8(b)]. (**b**) By gradually increasing $V$ toward –0.05 V, the edge level of the V.B. of the p-Semi enters the gap region of the SC. Then, an injected electron from the p-Semi to SC is Andreev-reflected (red arrow); because there are no quasiparticle states in the SC gap region, the electron is reflected back into the p-Semi side as a hole (empty dot).[21,44,45] The probability of the Andreev reflection (AR) is highest when the edge of the electron-rich V.B. of the p-Semi corresponds to the $\varepsilon_F$ of the SC, i.e., at $V$ = –0.05 V. The SC-related tunneling has already been confirmed by the $V^2$-proportional *dI/dV* in the voltage region denoted as (I) in Fig. 8(b). Additionally, by increasing $V$ from –0.85 V to –0.05 V, both tunneling of holes and electrons proceed in the direction to weaken $E_D$ (i.e., the direction to decrease the carrier density of holes and electrons at the SC and p-Semi sides of the Schottky interface, respectively). Thus, $E_D$ is minimized at $V$ = –0.05 V (i.e., when AR is strongest), which is consistent with the *C*–*V* result in Fig. 8(a). (**c**) When a subsequent increase in $V$ makes the Fermi level of the p-Semi lower than the $\varepsilon_F$ of the SC, the electron density at the p-Semi side of the interface starts to increase. Thus, $E_D$ is increased, which results in the inversion layer being observed in the *C*–*V* curve in the range of –0.05 < $V$ < +1.05 V in Fig. 8(a). In this bias voltage region, AR still occurs; however, solid arrows are not depicted to avoid a complicated illustration. (**d**) When $V$ reaches +1.05 V, where the edge level of the C.B. of the p-Semi corresponds to the $\varepsilon_F$ of the SC, the strongest AR is achieved again. That is, the probability of electrons reflection, which is induced by the injection of holes from the p-Semi to SC, is highest. The result is consistent with the observed *dI/dV* peak at $V$ = +1.05 V in Fig. 8(b). At the same time, the reflected electrons form the carrier distribution to maximize $E_D$. Thus, the *C*–*V* curve has shown the local maximum at $V$ = +1.05 V in Fig. 8(a). AR lasts until the edge level of the C.B. of the p-Semi corresponds to that of the V.B. of the SC, i.e., for the voltage range of +1.05 < $V$ < +1.85 V. The SC-related

tunneling has been confirmed by the $V^2$-proportional *dI/dV* in the voltage region denoted as (III) in Fig. 8(b). (**e**) For $V > +1.85$ V, the injected holes show ohmic tunneling, which is consistent with the *dI/dV* result for the same voltage region in Fig. 8(b). Because of the large bias voltage for which the polarity is opposite to that of $E_D$, *C* decreases in these voltage regions, as confirmed in Fig. 8(a). Thus, every feature of *C*–*V* [Fig. 8(a)] and *dI/dV*–*V* results [Fig. 8(b)] is completely included in this p-Semi–SC semiconductor model.

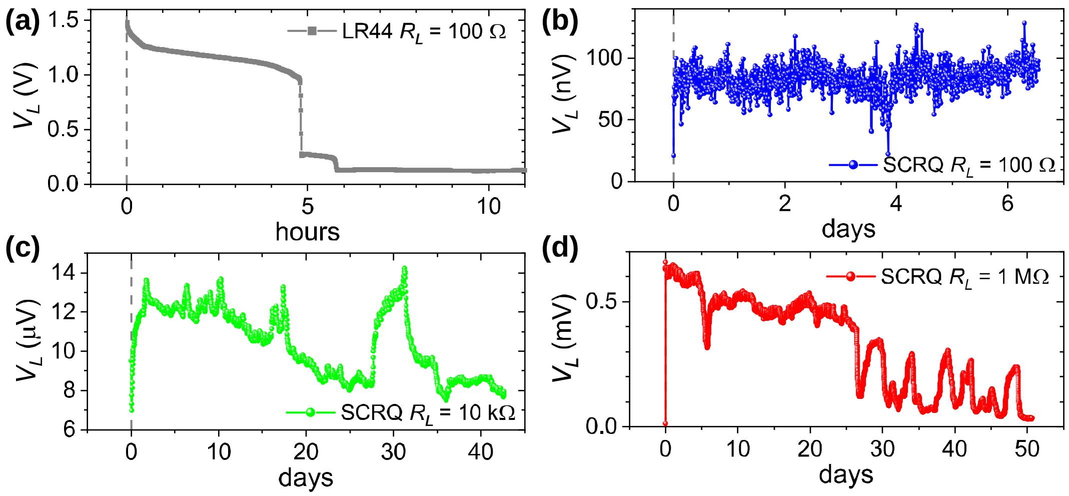


**Figure S4. Time evolution of $V_L$ in the atmosphere.** (**a**) Discharge test of an alkaline button cell (LR44, Panasonic) for $R_L$ = 100 Ω, which verifies the experimental setup. (**b**, **c**, and **d**) Discharge tests of the SCRQ for three different $R_L$ of 100 Ω, 10 kΩ, and 1 MΩ, respectively. Details of the measurements can be found in the Materials and Methods section "*Electrical measurements in the atmosphere.*"

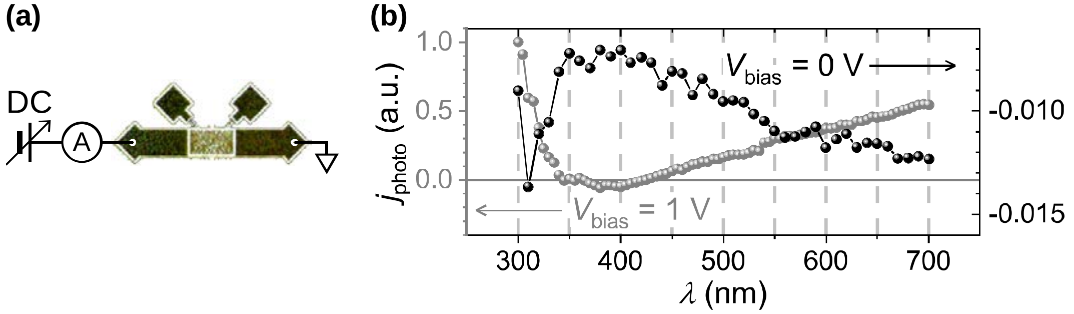


**Figure S5. Vis-spectral response of the SCRQ in the atmosphere.** The SCRQ was positioned in a custom-made spectral sensitivity characterization system (Bunkoukeiki), and the photocurrent density $j_{photo}$ at a constant DC bias voltage $V_{bias}$ was measured by the two-probe method using a source meter (2400, Keithley). (**a**) DC-voltage-biased SCRQ configuration used in this measurement. (**b**) Vis-spectral response of the SCRQ. The irradiating photon wavelength $\lambda$ ranges from 300 nm to 700 nm, and $j_{photo}$ (arbitrary unit) at $V_{bias}$ = 0 V (black) and +1 V (gray) are shown in the right and left axis, respectively; both $j_{photo}$ are normalized by the $j_{photo}$ value of $V_{bias}$ = +1 V at $\lambda$ = 300 nm. The reversed signs of $j_{photo}$ for $V_{bias}$ = 0 V and +1 V indicate that the oppositely charged carrier plays the main role in $j_{photo}$ for each biased voltage. For both $V_{bias}$, $|j_{photo}|$ forms a concave peak at $\lambda \sim 400$ nm (i.e., $h\nu \sim 3.1$ eV) distributed from 350 nm to 450 nm (i.e., $h\nu$: 3.5–2.7 eV). That is, $|j_{photo}|$ is suppressed in this region of $\lambda$. An increase of $|j_{photo}|$ in the range of $\lambda$ < 350 nm is due to the UV-vis absorption edge of the naturally oxidized surface of the sample, although a usual $NbO_x$ film never emits photocurrent.[62]

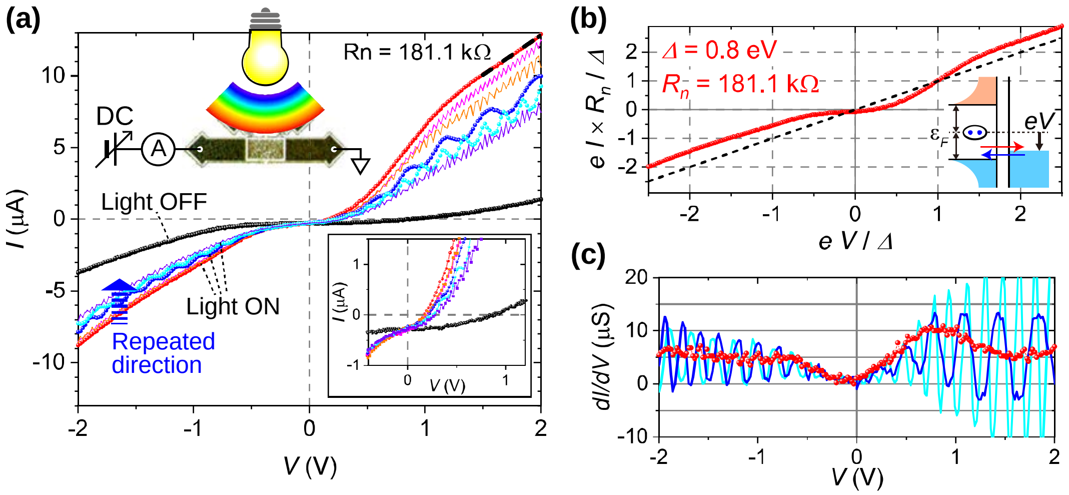


**Figure S6. SCRQ under intense Vis-light illumination in the atmosphere.** Under intense Vis-light illumination, the transport current of the DC-voltage-biased SCRQ was measured using the two-probe method; a chip LED (SG-325, Gentos) with a brightness of 150 lm, which was set approximately 5-cm apart from the SCRQ, and the SMU (B2911A, Keysight) were used as the white light source and the DC voltage source, respectively. (**a**) DC-voltage-dependent transport current in the SCRQ. After the *I–V* measurement without illumination (black symbol), the DC voltage cycle in the range of ±2 V was continuously repeated 20 times under the white light illumination (colored symbols): the first *I–V* curve, red; the 20th, purple; only the characteristic ones are shown here. The transport current is increased under the illumination, and the envelope[48] of the *I–V* curves is formed by sweeping voltage. Inset, zoomed-in plot; despite the illumination, current flows through the SCRQ even at zero-bias voltage. (**b**) Normalized *I–V* curve of the first voltage cycle in (a). In accordance with the procedure of Blonder *et al.*,[45] the *x* and *y* axes are normalized by $\Delta/e$ and $\Delta/eR_n$, respectively, where $\Delta$ is 0.8 eV, and $R_n$ is 181.1 kΩ as indicated by the black broken line in (a). The black dotted line in (b) is the reference line of $I = V/R_n$. For $eV > \Delta$, the photocurrent (red) differs in a constant amount from the reference line. The so-called excess current $I_{exc}$ has the amount of $eI_{exc}R_n / \Delta \sim 0.5$. According to Blonder *et al.*,[45] the barrier strengths is $Z \sim 0.8$, which indicates that the p-Semi–SC interface in this regime, along with the interface between the SCRQ and the normal-metal Nb electrodes, is sufficiently barrier-free to observe carrier tunneling. Inset, schematic diagram of the tunneling process between an SC and a normal-metal Nb electrode. (**c**) *dI/dV vs. V* plots obtained from (a); only the first (red), 12th (blue), and 14th (cyan) voltage cycles are shown here [those of all other voltage cycles can be found in Fig. S7]. For the first voltage cycle (red), the *dI/dV* is strongest at $V = \Delta/e$ (0.8 V), and the value is twice than that in the normal region. Thus, the validity of $\Delta$ and AR are confirmed. Furthermore, the *dI/dV* curves periodically oscillate[46] while sweeping voltage. In conclusion, the SCRQ in this regime (i.e., under intense Vis-light illumination) shows the CB of 2*e*–*e* parity effect.[46–51]

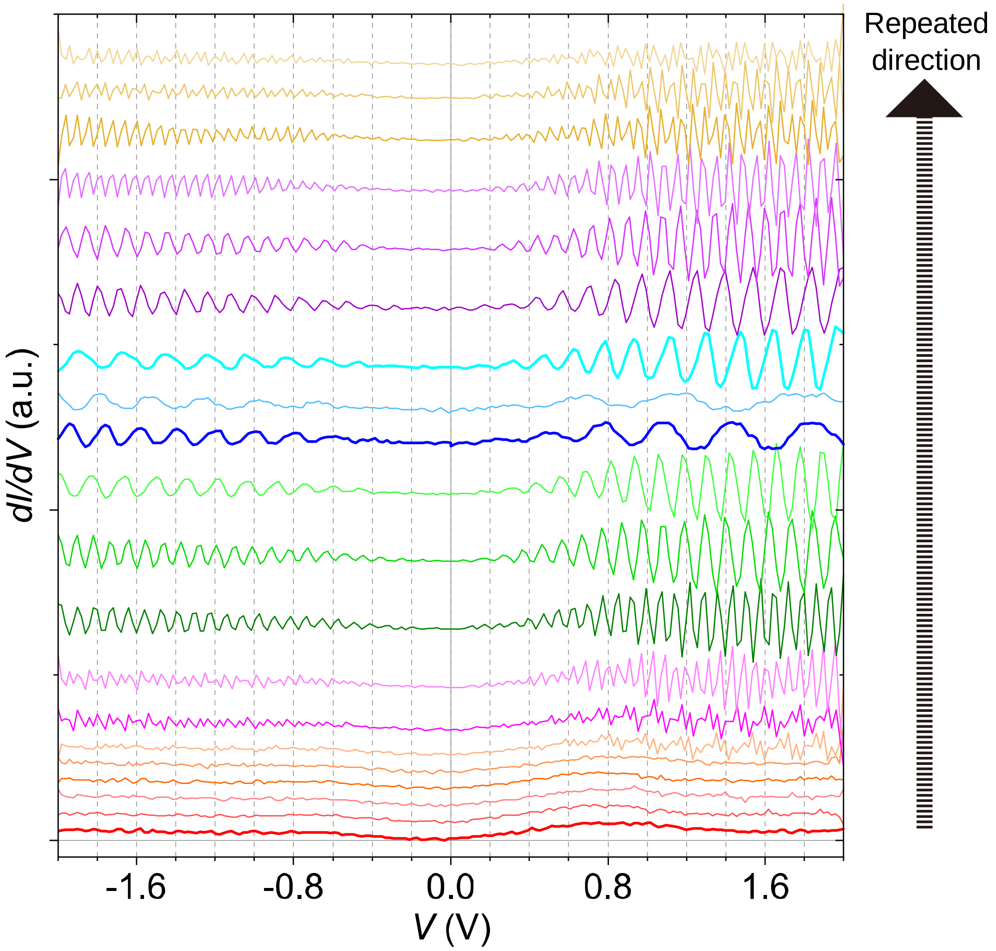


**Figure S7. *dI/dV*–*V* curves of all voltage cycles related to Fig. S6.** The measurement was repeated by sweeping the DC voltage for 20 cycles under the white light illumination, as explained in Fig. S6. The abruptly shifted curve in the *y*-axis from the bottom to the top corresponds to the first to 20th cycles, respectively. The thick red, blue, and cyan curves are already shown in Fig. S6(c). With an increase in the voltage cycles, the period of the *dI/dV* oscillation changes, and the doubly changed periodicity of the transported current can be confirmed by comparing the 12th (blue) and 14th cycle (cyan) in the positive voltage region, which indicates the 2*e* and *e* periodic pair currents in the CB regime. Conventionally, the 2*e*–*e* parity effect was observed in the gated SC island employing the double-JJ configuration, and the conventional even–odd symmetry breaker was the temperature;[50] that is, the thermally fluctuated $\varDelta$, and $E_C$ which was provided by the gate voltage, competed with each other. In this study, on the other hand, both $\varDelta$ and $E_g$ of the SC and the p-Semi, respectively, that are inherent in the SCRQ, are much larger than the thermal energy $k_BT$ at room temperature; thus, the temperature is not the symmetry breaker. Instead, charging, which is easily achieved by a simple connection of a two-probe DC bias source to the SCRQ, fluctuates $E_C$ of each elementary JJ, which breaks the symmetry.

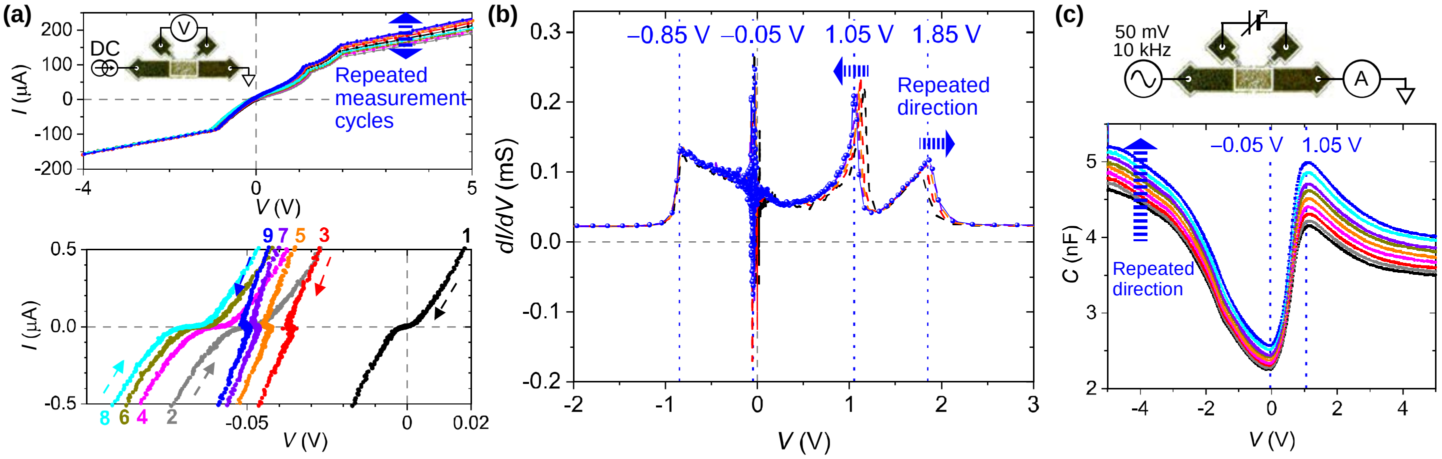


**Figure S8. All *dI/dV–V* and *C–V* curves of the SCRQ in the QPS regime, related to Fig. 8.** (**a**) Direct-current-dependent electrical characteristics of the SCRQ in the atmosphere. A direct current cycle was repeatedly applied. The *x* and *y* axes are exchanged for convenience. Lower panel, zoomed-in plot near the origin; denoted colored numbers, the number of repeated current cycles; broken arrows, direction of current sweeping. That is, odd and even numbers indicate that the current was swept from positive to negative and vice versa, respectively. By repeatedly sweeping current, the voltage crossing the axis of $I$ = 0 μA shifts to non-zero values. (**b**) *dI/dV vs. V* obtained from (a); only odd-cycle results are shown. Broken arrows denote the direction of an increase in the number of cycles; from the first (black) to the ninth (blue). Two peaks at $V$ = +1.05 and +1.85 V distinctly shift to the lower and higher values, respectively, by increasing the number of the current cycles, which is the nonequilibrium SC phenomenon known as the *enhancement of Δ by the extraction of quasiparticles*.[21,52] As shown, the peaks are shifted in the direction for $\Delta$ to be enhanced (broken arrows). Chi and Clarke[52] have experimentally demonstrated the enhancement of $\Delta$ using the Al-$Al_2O_3$-Al-$Al_2O_3$-Al tunnel junction, two energy gaps of which are different. The tunneling of quasiparticles from the SC with $\Delta_1$ to the adjacent SC with a larger gap $\Delta_2$ leads to a decrease in the quasiparticle density in the former SC, and consequently, the quasiparticles are "cooled" (i.e., $\Delta_1$ is enhanced). The following two requirements are essential to achieve the enhancement in $\Delta$: a large energy gap beside an SC and a junction configured to extract both an electron and a hole.[21] The SCRQ satisfies these two requirements [see Fig. 8(c)]. Thus, $\Delta$ is enhanced by the tunneling of quasiparticles from the SC to p-Semi. (**c**) *C–V* results of the SCRQ in the atmosphere. A DC voltage cycle from –5 V to +5 V was repeated nine times; the direction of an increase in the number of the voltage cycles is denoted by the broken arrow. By increasing the number of the voltage cycles, the total capacitance $C$ is increased to some extent, which is due to the charging effect caused by the voltage source. For the *C–V* and *dI/dV–V* curves in Fig. 8(a) and 8(b), respectively, the results of the ninth cycles (blue) in (c) and (b) are used. Details of the measurements can be found in the Materials and Methods section "*Electrical measurements in the atmosphere.*"

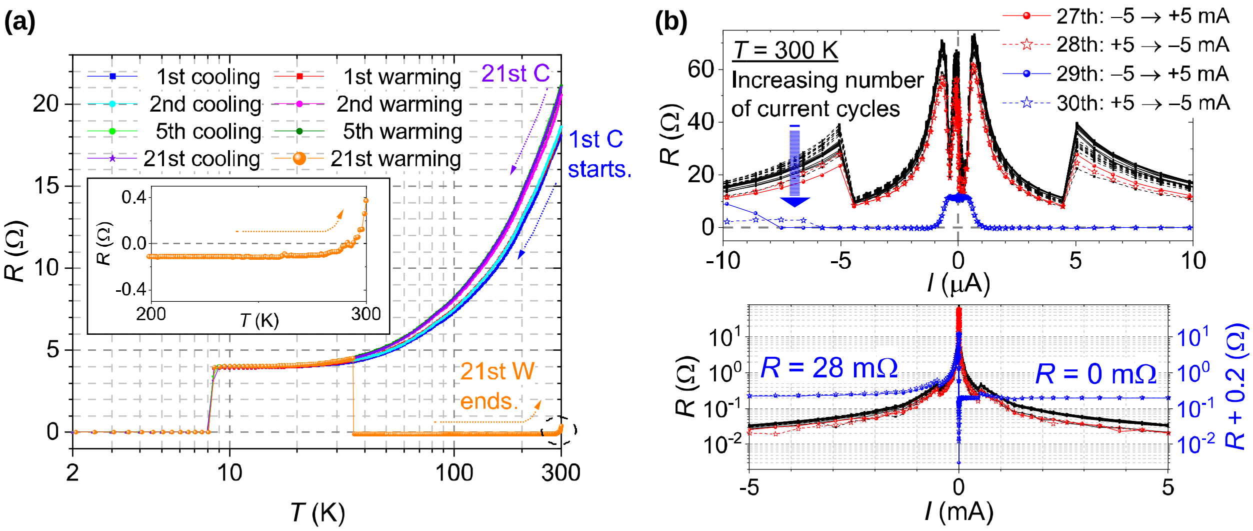


**Figure S9. Role of charging in making RTSC.** (**a**) *R*–*T* curves of a PnC–Nb sample of the same design as those reported in this study, obtained in zero magnetic field; only the first, second, fifth, and 21st cycles are shown here [all other *R*–*T* cycles can be found in Fig. S10]. Inset, zoomed-in plot of the final 21st warming process. The resistance decreases to a nearly zero negative value between 30 K and 40 K, and the value is maintained for a while; however, the resistance slightly increases just before 300 K. (**b**) Resistance profile of the near-miss RTSC obtained after completing the *R*–*T* cycles in (a). A pulsed current in the range of ±5 mA was repeatedly applied at 300 K in zero magnetic field. Upper panel, zoomed-in plot; the broken arrow indicates the direction to increase the number of the current cycles. Lower panel, logarithmic display; for the 29th and 30th cycles (blue), the logarithmic values are obtained by adding 0.2 Ω to *R* in advance as indicated in the right axis; otherwise, the entire curves cannot be displayed owing to the negative resistance in the current range from +1 to +100 μA. The resistance gradually decreases with the increase in the number of the current cycles. Finally, after the 29th cycle, the resistance decreased to zero for a certain current range. For this measurement, the resistance bridge board installed in the PPMS was used, which was operated in the AC drive mode, and the number of readings taken was 10.

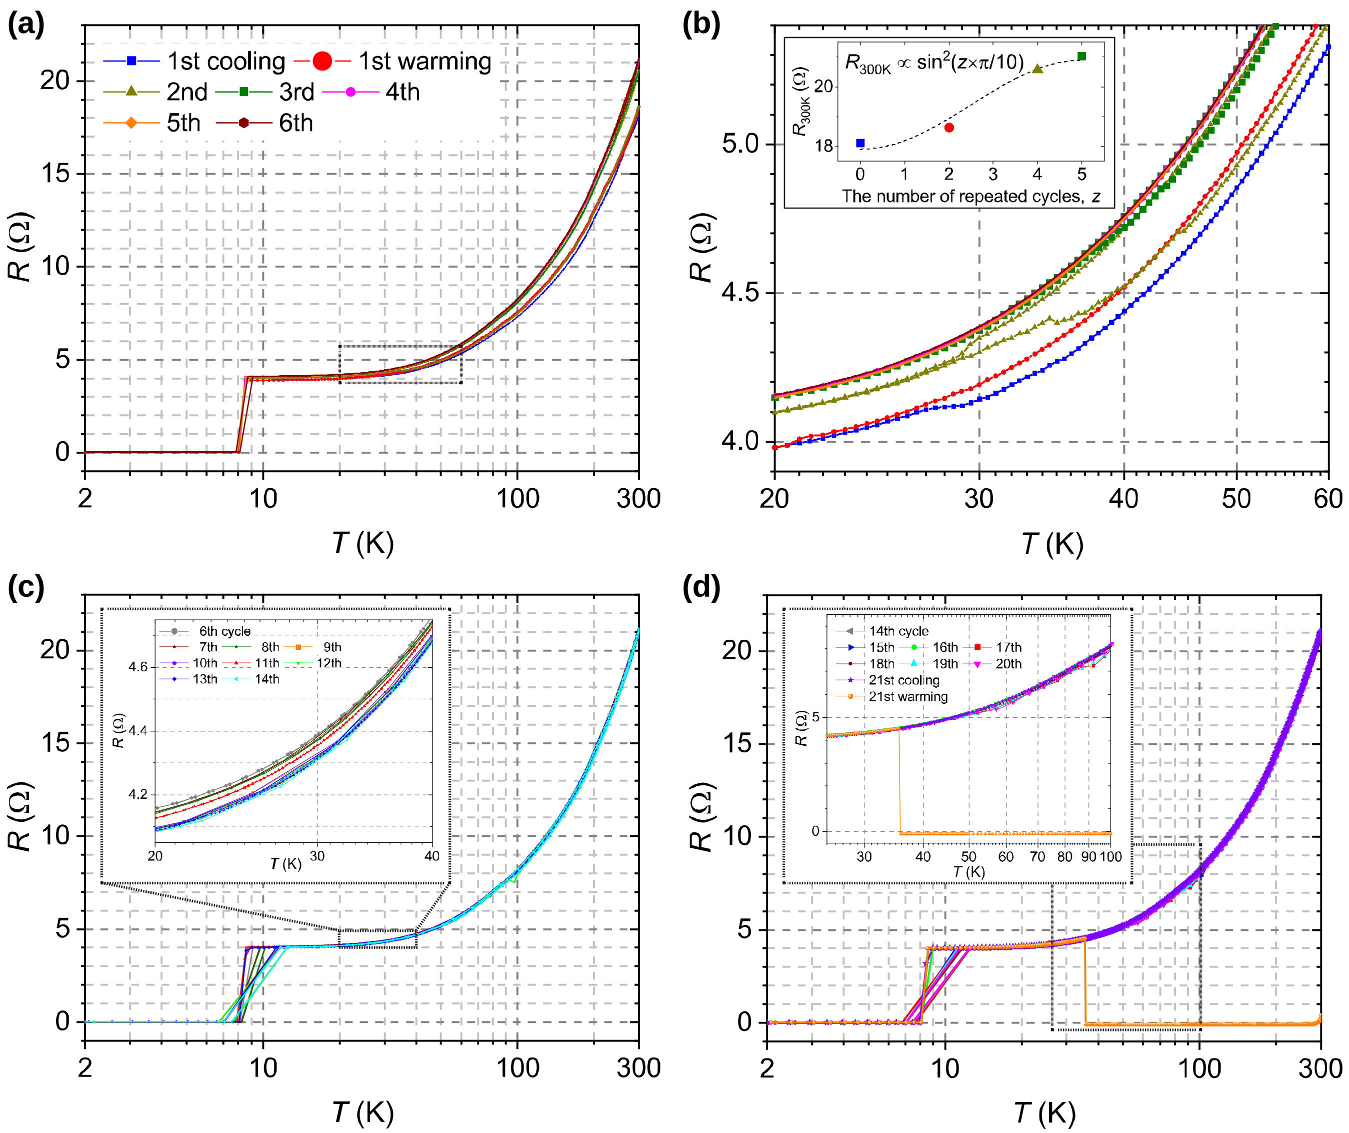


**Figure S10. *R*–*T* cycles which result in the near-miss RTSC.** (**a**) First to sixth temperature cycles. (**b**) Zoomed-in plot of the region surrounded by the black dashed square in (a). An abnormal increase in the resistance is confirmed between 20 K and 60 K, but the obvious non-retraced behavior is confirmed only for the first three cycles. The resistances at 300 K of the first cooling process (blue), first warming process (red), second warming process (yellow), and third warming process (green) are plotted in the inset. By assuming that two electrons at once occupy the *d* orbitals during the first and second cycles, the resistances follow the Friedel sum rule. (**c**) Sixth to the 14th cycle. As shown in the inset, the obvious non-retraced behavior is lost for each temperature cycle, but the entire *R*–*T* curve goes up and down, which is identical to that shown in Fig. S1(c). (**d**) The rest of the *R*–*T* cycles. Inset, zoomed-in plot. In the 19th and 20th cycles, *R*–*T* curves exhibit unstable behavior at high temperatures (50–120 K), which is identical to that shown in Fig. S1(d). See Table S4 for the cooling–warming procedures of this measurement.

**Table S4. Cooling–warming procedures for Fig. S10**

| Cycle number | Cooling–warming rate and temperature approaching mode* | | Elapsed time |
|---|---|---|---|
| 1st ~ 4th | 300 → 60 K: 1 K/min | S | 18 ~ 19 hrs/cycle |
| | 60 → 2 K: 0.5 K/min | F | |
| | 2 → 60 K: 0.5 K/min | F | |
| | 60 → 300 K: 1 K/min | S | |
| 5th | 300 → 50 K: 1 K/min | S | 17.6 hrs |
| | 50 → 25 K: 0.25 K/min | F | |
| | 25 → 2 K: 0.5 K/min | S | |
| | 2 → 25 K: 0.5 K/min | S | |
| | 25 → 50 K: 0.25 K/min | F | |
| | 50 → 300 K: 1 K/min | S | |
| 6th | 300 → 2 K: 1 K/min | S | 9.9 hrs |
| | 2 → 300 K: 1 K/min | S | |
| 7th ~ 8th | 300 → 2 K: 2 K/min | S | 5 ~ 6 hrs/cycle |
| | 2 → 300 K: 2 K/min | S | |
| 9th | 300 → 2 K: 5 K/min | S | 2.4 hrs |
| | 2 → 300 K: 5 K/min | S | |
| 10th | 300 → 2 K: 5 K/min | S | 10.4 hrs |
| | 2 → 25 K: 0.5 K/min | S | |
| | 25 → 50 K: 0.25 K/min | F | |
| | 50 → 300 K: 1 K/min | S | |
| 11th | 300 → 50 K: 1 K/min | S | 18.0 hrs |
| | 50 → 25 K: 0.25 K/min | F | |
| | 25 → 2 K: 0.5 K/min | S | |
| | 2 → 25 K: 0.5 K/min | S | |
| | 25 → 50 K: 0.25 K/min | F | |
| | 50 → 300 K: 1 K/min | S | |
| 12th | 300 → 2 K: 5 K/min | S | 2.4 hrs |
| | 2 → 300 K: 5 K/min | S | |
| 13th | 300 → 2 K: 5 K/min | S | 12.3 hrs |
| | 2 → 20 K: 0.5 K/min | S | |
| | 20 → 60 K: 0.25 K/min | F | |
| | 60 → 300 K: 1 K/min | S | |
| 14th ~ 15th | 300 → 2 K: 5 K/min | S | 2 ~ 3 hrs/cycle |
| | 2 → 300 K: 5 K/min | S | |
| 16th | 300 → 50 K: 1 K/min | S | 17.9 hrs |
| | 50 → 25 K: 0.25 K/min | F | |
| | 25 → 2 K: 0.5 K/min | S | |
| | 2 → 25 K: 0.5 K/min | S | |
| | 25 → 50 K: 0.25 K/min | F | |
| | 50 → 300 K: 1 K/min | S | |
| 17th | 300 → 2 K: 5 K/min | S | 2.4 hrs |
| | 2 → 300 K: 5 K/min | S | |
| 18th | 300 → 2 K: 5 K/min | S | 10.9 hrs |
| | 2 → 25 K: 0.5 K/min | S | |
| | 25 → 50 K: 0.25 K/min | S | |
| | 50 → 90 K: 1 K/min | S | |
| | 90 → 110 K: 0.25 K/min | F | |
| | 110 → 300 K: 1 K/min | S | |
| 19th ~ 20th | 300 → 2 K: 5 K/min | S | 2 ~3 hrs/cycle |
| | 2 → 300 K: 5 K/min | S | |
| 21st | 300 → 50 K: 1 K/min | S | 19.0 hrs |
| | 50 → 25 K: 0.25 K/min | F | |
| | 25 → 2 K: 0.5 K/min | S | |
| | 2 → 25 K: 0.5 K/min | S | |
| | 25 → 50 K: 0.25 K/min | F | |
| | 50 → 90 K: 1 K/min | S | |
| | 90 → 110 K: 0.25 K/min | S | |
| | 110 → 300 K: 1 K/min | S | |

We performed the measurements in zero magnetic field using the PPMS. The PPMS was operated in the AC drive mode using the standard calibration mode. The amplitude of the square-wave excitation current was ±10 μA. At each resistance measurement, the number of readings was 25. See Materials and Methods section "*R–T measurements*" for details.

*Letters "S" and "F" after each cooling–warming rate indicate that the resistance is measured by sweeping or fixing the temperature, respectively.

**MFM Results**

The conventional techniques to demonstrate SC diamagnetism or the Meissner effect for bulk materials is to investigate how the magnetic susceptibility of a specimen depends on the temperature and magnetic field. However, the RTSC sample of this study is a physically microfabricated PnC–Nb, in which diamagnetism created by the massive silicon (Si) substrate that supports the tiny RTSC film veils any SC magnetic susceptibility.

Instead, magnetic force microscopy (MFM) is adopted in this study. The magnetized tip of a cantilever oscillating above the surface of the sample detects stray magnetic fields near the sample. The MFM measurements were performed in the atmosphere (i.e., at room temperature, in a terrestrial magnetic field, and under atmospheric pressure) using SPM-9700 (Shimadzu) with a low-noise option, which employed an optical-lever AFM head and a tube-piezoelectric scanner. The cantilever with a cobalt-chromium coating (MESP, Veeco), with tip radius, resonant frequency, and force constant of 35 nm, 71.5 kHz, and typically 2 N/m, respectively, was selected. A sample was mounted on the sample stage without glue. Figure S11(a) and (b) show CCD images of a metallic PnC–Nb and an RTSC, respectively, set in the apparatus. The MFM cantilever is also shown; the area of 30 × 30 $\mu m^2$ in the vicinity of the tip of the cantilever was scanned. The MFM tip moved in the horizontal *x*-direction, and the *x*-line scan continued in the vertical *y*-direction; each *x*-line scan was performed at a scan speed of 1 Hz. Because the suspended thin film structure of the PnC–Nb makes it challenging to maintain a constant distance between the tip and the sample surface, each MFM line scan was executed with the MFM tip kept at a constant height.

Figure S11(c) shows an MFM image of the as-fabricated PnC–Nb prior to temperature cycling (thus, the sample is in a normal metallic state). A Nb island and several Nb bridges are visible. In case of such nonmagnetic metallic films without any current passing through them, the magnetic flux that originates from the oscillating magnetized tip penetrates the film, inducing an eddy current in the film, and a magnetic force is generated by the eddy current; consequently, the magnetic force causes a phase delay of the oscillation of the magnetized tip, which results in an MFM image.[63] Thus, the visible Nb island and bridges in the MFM image in Fig. S11(c) indicate that the magnetic flux penetrates the film, confirming that the sample is a normal metal. Black shadows in the MFM image indicate that the magnetized tip touches the surface of the PnC–Nb that is slightly wavy. The focused phase magnitude of the MFM image is set to 25 degrees, which is common to all following MFM images. Also, neither data calculations nor image processing is

performed for all the MFM images.

Subsequently, the RTSC sample was scanned by MFM. The original purpose of this experiment was to see whether the magnetic flux could be trapped within the periodic thru-holes distributed in the RTSC film or not. Therefore, just before beginning the MFM measurement, the RTSC sample was mounted on a magnet with a magnetic flux density of 0.2 T for 20 minutes. As shown in Fig. S11(d), during the scan, the MFM tip is much closer to the surface of the sample than the case for the metallic PnC–Nb in Fig. S11(c), which can be determined from the severe black shadows in Fig. S11(d). Nevertheless, neither Nb islands nor bridges are discernible in the MFM image [Fig. S11(d)]. That is, the magnetic flux does not penetrate the film itself; indeed, the sample is not in a normal metallic state but in the RTSC state as expected. Yet the MFM image is wholly absent; that is, the magnetic flux is not trapped within the thru-holes. Thus, the thru-hole is not a mere defect, but rather, it provides center-of-mass motion of Cooper pairs. In other words, the circulating supercurrent flowing through the Mott ring [Fig. 5] rejects the penetration of any external magnetic field. Thus, our consideration of the type-I superconductivity of the RTSC in this study is supported by this MFM measurement.

Moreover, after the height of the MFM tip was further decreased by 300 nm, the RTSC was scanned again. In the beginning of the scanning, the phase ranged approximately 60–85 degrees only [Fig. S11(e)], which is the same as Fig. S11(d). However, immediately after the moving MFM tip severed the bridge, the MFM phase drastically shifted to an anomalous value ranging approximately from –147 to –122 degrees [Fig. S11(f)]. (Because the MFM image is obtainable only after the scan is completed from top to bottom, the anomalous phase peak value is already shown in the scale bar in Fig. S11(e).) Although the interpretation of this result is not straightforward, we assume that the severance of a bridge, which breaks a Mott ring, causes the sudden appearance of the MFM image. At least, these MFM results do not contradict the principle of the Mott ring [Fig. 5], the experimental result of $\xi$ obtained from the PSC phenomenon [Fig. 7(b)], and the estimation of $\lambda_{\perp}$ that supports the type-I superconductivity of this 2D RTSC system.

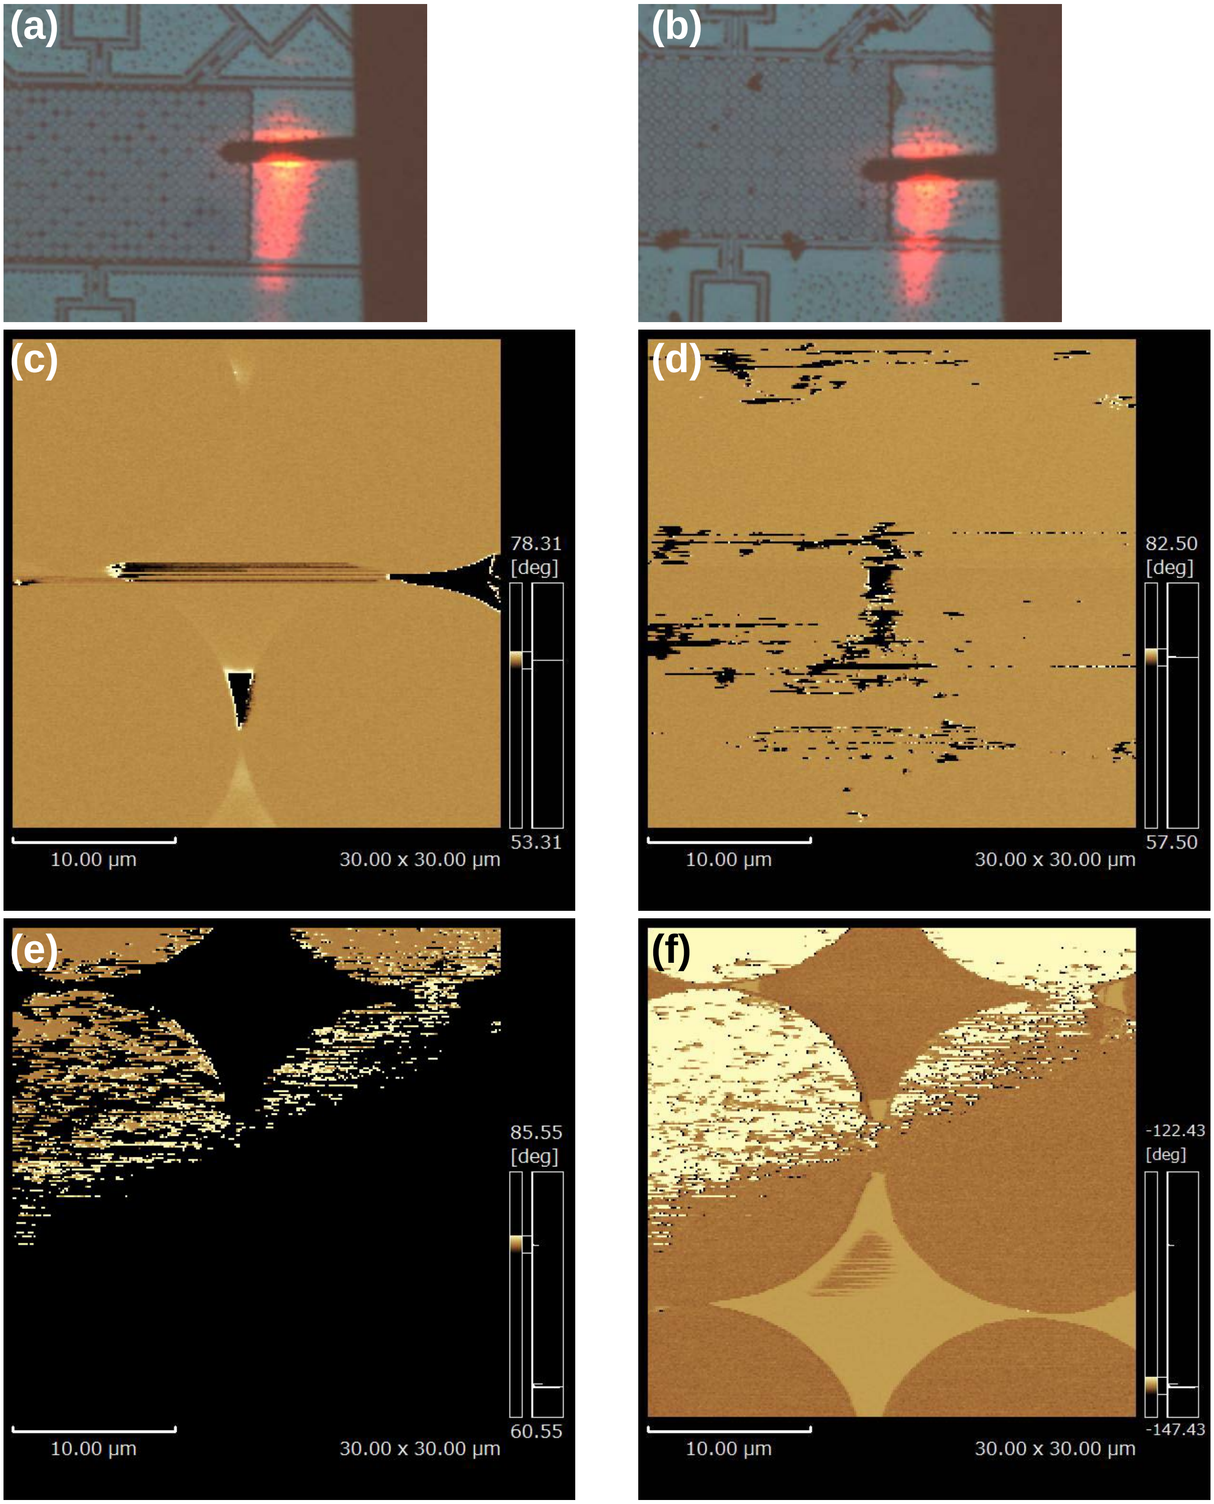


**Figure S11. MFM results.** (**a** and **b**) CCD images of a metallic PnC–Nb and an RTSC, respectively, set in the MFM apparatus. (**c** and **d**) MFM images of the metallic PnC–Nb and the RTSC, respectively. (**e**) MFM image of the RTSC after decreasing the height of the MFM tip by 300 nm, subsequently to the measurement of (d). (**f**) The same MFM image in (e), focusing on the anomalous phase peak that appears just after the moving MFM tip in the horizontal direction severs a bridge. For all the MFM images, the focused phase magnitudes are set to 25 degrees, and neither data calculations nor image processing is performed.

**References**


[1] H. K. Onnes, *The resistance of pure mercury at helium temperatures*, Commun. Phys. Lab. Univ. Leiden **120b**, 1479–1481 (1911).

[2] J. Bardeen, L. N. Cooper, and J. R. Schrieffer, *Microscopic Theory of Superconductivity*, Phys. Rev. **106**, 162–164 (1957).

[3] J. G. Bednorz and K. A. Müller, *Possible high $T_C$ superconductivity in the Ba-La-Cu-O system*, Z. Phys. B **64**, 189–193 (1986).

[4] P. W. Anderson, *Basic Notions of Condensed Matter Physics* (Benjamin-Cummings Publishing, Menlo Park, CA, 1984).

[5] P. W. Anderson, *The Resonating Valence Bond State in $La_2CuO_4$ and Superconductivity*, Science **235**, 1196–1198 (1987).

[6] P. W. Anderson, *Is there glue in cuprate superconductors?* Science **316**, 1705–1707 (2007).

[7] H. Aoki, *Introduction to Superconductivity* (Shokabo, Tokyo, 2014).

[8] H. Shiba, *Physics of Correlated Electron Systems* (Iwanami Shoten, Tokyo, 2016).

[9] H. Fukuyama and J. Akimitsu, *Handbook of Superconductivity* (Asakura Shoten, Tokyo, 2009).

[10] D. J. Scalapino, *The case for $d_{x2-y2}$ paring in the cuprate superconductors*, Physics Reports **250**, 329–365 (1995).

[11] E. Snider, N. Dasenbrock-Gammon, R. McBride, M. Debessai, H. Vindana, K. Vencatasamy, K. V. Lawler, A. Salamat, and R. P. Dias, *Room-temperature superconductivity in a carbonaceous sulfur hydride*, Nature **586**, 373–377 (2020).

[12] A. P. Drozdov, M. I. Eremets, I. A. Troyan, V. Ksenofontov, and S. I. Shylin, *Conventional superconductivity at 203 kelvin at high pressures in the sulfur hydride system*, Nature **525**, 73–76 (2015).

[13] M. Somayazulu, M. Ahart, A. K. Mishra, Z. M. Geballe, M. Baldini, Y. Meng, V. V. Struzhkin, and R. J. Hemley, *Evidence for Superconductivity above 260 K in Lanthanum Superhydride at Megabar Pressures*, Phys. Rev. Lett. **122**, 027001 (2019).

[14] D. V. Semenok, A. G. Kvashnin, A. G. Ivanova, V. Svitlyk, V. Yu. Fominski, A. V. Sadakov, O. A. Sobolevskiy, V. M. Pudalov, I. A. Troyan, and A. R. Oganov, *Superconductivity at 161 K in thorium hydride $ThH_{10}$: Synthesis and properties*, Mater. Today **33**, 36–44 (2020).

[15] P. Monthoux and G. G. Lonzarich, *p-wave and d-wave superconductivity in quasi-two-dimensional metals*, Phys. Rev. B **59**, 14598–14605 (1999).

[16] R. Arita, K. Kuroki, and H. Aoki, *Spin-fluctuation exchange study of superconductivity in two- and three-dimensional single-band Hubbard models*, Phys. Rev. B **60**, 14585–14588 (1999).

[17] T. Scheike, W. Böhlmann, P. Esquinazi, J. Barzola-Quiquia, A. Ballestar, and A. Setzer, *Can Doping*

*Graphite Trigger Room Temperature Superconductivity? Evidence for Granular High-Temperature Superconductivity in Water-Treated Graphite Powder*, Adv. Mater. **24**, 5826–5831 (2012).
[18] C. E. Precker, P. D. Esquinazi, A. Champi, J. Barzola-Quiquia, M. Zoraghi, S. Muiños-Landin, A. Setzer, W. Böhlmann, D. Spemann, and J. Meijer, *Identification of a possible superconducting transition above room temperature in natural graphite crystals*, New J. Phys. **18**, 113041 (2016).
[19] E. Šimánek, *Inhomogeneous Superconductors* (Oxford University Press, New York, NY, 1994).
[20] R. M. Bradley and S. Doniach, *Quantum fluctuations in chains of Josephson junctions*, Phys. Rev. B **30**, 1138–1147 (1984).
[21] M. Tinkham, *Introduction to Superconductivity*, 2nd ed. (Dover Publications, Mineola, NY, 2004).
[22] J. R. Phillips, H. S. J. van der Zant, J. White, and T. P. Orlando, *Influence of induced magnetic fields on the static properties of Josephson-junction arrays*, Phys. Rev. B **47**, 5219–5229 (1993).
[23] N. Zen, *Phonon-engineered Nb film as a Mott-insulating tunnel-junction network*, AIP Adv. **9**, 095023 (2019).
[24] I. Maasilta and A. J. Minnich, *Heat under the microscope*, Phys. Today **67**, 27–32 (2014).
[25] M. Maldovan, *Phonon wave interference and thermal bandgap materials*, Nature Mater. **14**, 667–674 (2015).
[26] M. Date, *Graduate School–Condensed Matter Physics 2* (Kodansha, Tokyo, 1997).
[27] J. Villain, M. Lavagna, and P. Bruno, *Jacques Friedel and the physics of metals and alloys*, C. R. Physique **17**, 276–290 (2016).
[28] N. Zen, *Raw Data from the Study of the Room-Temperature Superconductivity and Its Advanced Phase, Dryad Dataset*, https://doi.org/10.5061/dryad.qjq2bvqf3, submitted: November, **2020**.
[29] D. V. Averin, A. B. Zorin, and K. K. Likharev, *Bloch oscillations in small Josephson junctions*, Sov. Phys. JETP **61**, 407–413 (1985).
[30] T. A. Fulton, P. L. Gammel, D. J. Bishop, L. N. Dunkleberger, and G. J. Dolan, *Observation of combined Josephson and charging effects in small tunnel junction circuits*, Phys. Rev. Lett. **63**, 1307–1310 (1989).
[31] B. D. Josephson, *Possible new effects in superconducting tunnelling*, Phys. Lett. **1**, 251–253 (1962).
[32] V. Ambegaokar and A. Baratoff, *Tunneling between superconductors*, Phys. Rev. Lett. **11**, 104 (1963).
[33] J. Meyer and G. v. Minnigerode, *Instabilities in the transition curve of current-carrying one-dimensional superconductors*, Phys. Lett. **38A**, 529–530 (1972).
[34] J. E. Mooij and Yu. V. Nazarov, *Superconducting nanowires as quantum phase-slip junctions, Nature Phys.* **2**, 169–172 (2006).
[35] G. Rastelli, I. M. Pop, and F. W. J. Hekking, *Quantum phase slips in Josephson junction rings*, Phys. Rev. B **87**, 174513 (2013).

[36] A. Ergül, J. Lidmar, J. Johansson, Y. Azizoğlu, D. Schaeffer, and D. B. Haviland, *Localizing quantum phase slips in one-dimensional Josephson junction chains*, New J. Phys. **15**, 095014 (2013).

[37] A. Ergül, T. Weißl, J. Johansson, J. Lidmar, and D. B. Haviland, *Spatial and temporal distribution of phase slips in Josephson junction chains*, Sci. Rep. **7**, 11447 (2017).

[38] C. W. J. Beenakker, *Search for Majorana fermions in superconductors*, *arXiv Preprint*, arXiv:1112.1950, v2, submitted: April, **2012**.

[39] B. van Heck, A. R. Akhmerov, F. Hassler, M. Burrello, and C. W. J. Beenakker, *Coulomb-assisted braiding of Majorana fermions in a Josephson junction array*, New J. Phys. **14**, 035019 (2012).

[40] S. Vijay and L. Fu, *Physical implementation of a Majorana fermion surface code for fault-tolerant quantum computation*, Phys. Scr. **T168**, 014002 (2016).

[41] V. Mourik, K. Zuo, S. M. Frolov, S. R. Plissard, E. P. A. M. Bakkers, and L. P. Kouwenhoven, *Signatures of Majorana Fermions in Hybrid Superconductor-Semiconductor Nanowire Devices*, Science **336**, 1003–1007 (2012).

[42] P. Monthoux, A. V. Balatsky, and D. Pines, *Weak-coupling theory of high-temperature superconductivity in the antiferromagnetically correlated copper oxides*, Phys. Rev. B **46**, 14803–14817 (1992).

[43] K. Tanabe, Y. Hidaka, S. Karimoto, and M. Suzuki, *Observation of both pair and quasiparticle tunneling in intrinsic junction stacks fabricated on $Bi_2Sr_2CaCu_2O_{8+\delta}$ single crystals*, Phys. Rev. B **53**, 9348–9352 (1996).

[44] A. F. Andreev, *The Thermal Conductivity of the Intermediate State in Superconductors*, Sov. Phys. JETP **19**, 1228–1231 (1964).

[45] G. E. Blonder, M. Tinkham, and T. M. Klapwijk, *Transition from metallic to tunneling regimes in superconducting microconstrictions: Excess current, charge imbalance, and supercurrent conversion*, Phys. Rev. B **25**, 4515–4532 (1982).

[46] D. B. Haviland, Yu. Pashkin, and L. S. Kuzmin, *Measurement of the superconducting single electron transistor in a high impedance environment*, Physica B **203**, 347–353 (1994).

[47] R. J. Fitzgerald, S. L. Pohlen, and M. Tinkham, *Observation of Andreev reflection in all-superconducting single-electron transistors*, Phys. Rev. B **57**, R11073–11076 (1998).

[48] J. M. Hergenrother, M. T. Tuominen, and M. Tinkham, *Charge transport by Andreev reflection through a mesoscopic superconducting island*, Phys. Rev. Lett. **72**, 1742–1745 (1994).

[49] T. M. Eiles, M. H. Devoret, and J. M. Martinis, *Coulomb blockade of Andreev reflection in the NSN single-electron transistor*, Surf. Sci. **305**, 536–540 (1994).

[50] A. Amar, D. Song, C. J. Lobb, and F. C. Wellstood, *2e and e Periodic pair currents in superconducting coulomb-blockade electrometers*, Phys. Rev. Lett. **72**, 3234–3237 (1994).

[51] J. P. Pekola, J. J. Vartiainen, M. Möttönen, O.-P. Saira, M. Meschke, and D. V. Averin, *Hybrid single-electron transistor as a source of quantized electric current*, Nature Phys. **4**, 120–124 (2008).

[52] C. C. Chi and J. Clarke, *Enhancement of the energy gap in superconducting aluminum by tunneling extraction of quasiparticles*, Phys. Rev. B **20**, 4465–4473 (1979).

[53] K. Makino, K. Kato, Y. Saito, P. Fons, A. V. Kolobov, J. Tominaga, T. Nakano, and M. Nakajima, *Terahertz spectroscopic characterization of $Ge_2Sb_2Te_5$ phase change materials for photonics applications*, J. Mater. Chem. C **7**, 8209–8215 (2019).

[54] R. Abe and H. Shiba, *Low Temperature Materials Physics* (Baifukan, Tokyo, 1988).

[55] J.-P. Pouget, P. Alemany, and E. Canadell, *Donor–anion interactions in quarter-filled low-dimensional organic conductors*, Mater. Horiz. **5**, 590–640 (2018).

[56] E. Fermi, *Thermodynamics* (Prentice Hall, Upper Saddle River, NJ, 1937).

[57] P. A. M. Dirac, *The Principles of Quantum Mechanics*, 4th ed. (Oxford University Press, New York, NY, 1958).

[58] K. Sato, *First-order phase transition of a vacuum and the expansion of the Universe*, Mon. Not. R. Astron. Soc. **195**, 467–479 (1981).

[59] A. H. Guth, *Inflationary universe: A possible solution to the horizon and flatness problems*, Phys. Rev. D **23**, 347–356 (1981).

[60] Y. Nambu, *Quasi-particles and gauge invariance in the theory of superconductivity*, Phys. Rev. **117**, 648–663 (1960).

[61] P. W. Anderson, in *BCS: 50 Years* (Eds: L. N. Cooper, D. Feldman), World Scientific Publishing, Singapore **2011**.

[62] Y. Shan, Z. Zheng, J. Liu, Y. Yang, Z. Li, Z. Huang, and H. Jiang, *Niobium pentoxide: a promising surface-enhanced Raman scattering active semiconductor substrate*, NPJ Comput. Mater. **3**, 11 (2017).

[63] F. Wakaya, K. Oosawa, M. Kajiwara, S. Abo, and M. Takai, *Detection of nonmagnetic metal thin film using magnetic force microscopy*, Appl. Phys. Lett. **113**, 261601 (2018).
